# Supplementary material for: On Leveraging Encoder-only Pre-trained Language Models for Effective Keyphrase Generation
Source: arXiv:2402.14052 source file (2024-02-21)
Supplement: Supplementary file 1 [file all_results.tex]

\setlength{\tabcolsep}{4pt}
\begin{table*}[!ht]
    % \small
    \centering
    \resizebox{\linewidth}{!}{%
    \begin{tabular}{l | c | l l | l l | l l | l l | l l }
    \hline
    \multirow{2}{*}{Method} &
    \multirow{2}{*}{|M|} & \multicolumn{2}{c|}{\textbf{KP20k}} & \multicolumn{2}{c|}{\textbf{Inspec}} & \multicolumn{2}{c|}{\textbf{Krapivin}} & \multicolumn{2}{c|}{\textbf{NUS}} & \multicolumn{2}{c}{\textbf{SemEval}} \\
    & & F1@5 & F1@M & F1@5 & F1@M & F1@5 & F1@M & F1@5 & F1@M & F1@5 & F1@M\\
    \hline
    \multicolumn{8}{l}{(keyphrase extraction baselines)} \\
    KP-Miner & - & 21.9 & \hfil - \hfil & 14.4 & \hfil - \hfil & 20.6 & \hfil - \hfil& 28.3 & \hfil - \hfil & 24.4 & \hfil - \hfil\\
    YAKE & - & 18.8 & \hfil - \hfil & 19.0 & \hfil - \hfil & 19.4 & \hfil - \hfil & 22.4 & \hfil - \hfil & 20.7 & \hfil - \hfil\\
    TextRank & - & 16.2 & \hfil - \hfil & 22.6 & \hfil - \hfil & 13.6 & \hfil - \hfil& 20.8 & \hfil - \hfil & 18.7 & \hfil - \hfil \\
    PositionRank & - & 18.9 & \hfil - \hfil& 30.4 & \hfil - \hfil & 18.9 & \hfil - \hfil& 23.0 & \hfil - \hfil& 23.8 & \hfil - \hfil\\
    MultipartiteRank & - & 18.8 & \hfil - \hfil& 25.9 & \hfil - \hfil & 17.4 & \hfil - \hfil& 24.8 & \hfil - \hfil& 22.2 & \hfil - \hfil\\
    EmbedRank & - & 15.5 & \hfil - \hfil& 33.6 & \hfil - \hfil& 16.9 & \hfil - \hfil& 17.3 & \hfil - \hfil& 19.2 & \hfil - \hfil\\
    SIFRank+ & - & 20.0 & \hfil - \hfil & 35.1 & \hfil - \hfil& 19.6 & \hfil - \hfil& 25.5 & \hfil - \hfil& 24.8 & \hfil - \hfil\\
    \citet{liang-etal-2021-unsupervised} & - & 17.7 & \hfil - \hfil& 29.6 & \hfil - \hfil& 16.9 & \hfil - \hfil& 25.0 & \hfil - \hfil& 25.3 & \hfil - \hfil\\
    Kea & - & 19.4 &\hfil - \hfil& 12.7 & \hfil - \hfil& 16.0 & \hfil - \hfil& 23.6 & \hfil - \hfil& 15.5 & \hfil - \hfil\\
    \hline
    \multicolumn{6}{l}{(supervised keyphrase extraction)}  \\
    Transformer & 110M & 23.5$_6$ & 33.8$_4$ & 11.1$_3$ & 15.4$_5$ & 16.6$_{11}$ & 26.5$_{16}$ & 26.1$_{13}$ & 35.9$_{13}$ & 18.7$_7$ & 25.2$_7$ \\
    Transformer+CRF & 110M & 24.9$_{10}$ & 36.4$_6$ & 13.3$_{12}$ & 18.7$_{13}$ & 18.9$_{19}$ & 29.7$_{22}$ & 27.8$_{15}$ & 37.7$_{16}$ & 19.8$_{20}$ & 27.3$_{20}$ \\
    BERT-base & 110M & 27.9$_1$ & 38.9$_1$ & 12.8$_4$ & 17.4$_4$ & 20.7$_{11}$ & 30.2$_{17}$ & 30.9$_7$ & 41.0$_6$ & 21.8$_{11}$ & 28.5$_{13}$ \\
    BERT-base+CRF & 110M & 28.0$_2$ & 40.6$_3$ & 13.7$_5$ & 18.8$_9$ & 21.0$_3$ & 32.6$_{10}$ & 31.3$_9$ & 41.9$_{16}$ & 22.3$_6$ & 29.3$_{15}$  \\
    SciBERT & 110M & 28.6$_9$ & 40.5$_5$ & 13.1$_{11}$ & 17.8$_{13}$ & 19.9$_{12}$ & 30.3$_{13}$ & 29.7$_5$ & 39.0$_{13}$ & 20.0$_{22}$ & 26.3$_{30}$ \\
    SciBERT+CRF & 110M & 28.4$_{13}$ & 42.1$_{11}$ & 13.9$_{14}$ & 19.6$_{11}$ & 20.6$_{12}$ & 32.2$_{14}$ & 29.9$_{12}$ & 40.8$_{10}$ & 21.3$_{15}$ & 28.6$_{12}$  \\
    NewsBERT & 110M & 25.8$_6$ & 37.5$_5$ & 11.8$_4$ & 16.4$_3$ & 18.3$_6$ & 28.1$_{10}$ & 27.5$_{11}$ & 37.6$_{13}$ & 19.7$_2$ & 26.4$_7$ \\
    NewsBERT+CRF & 110M & 26.8$_3$ & 39.7$_1$ & 13.5$_4$ & 19.0$_8$ & 19.9$_{11}$ & 31.4$_{19}$ & 29.5$_{12}$ & 40.4$_{13}$ & 21.5$_5$ & 29.0$_6$ \\
    % RoBERTa-base & 125M & 27.9$_4$ & 39.4$_2$ & 13.9$_8$ & 18.9$_{12}$ & 19.1$_3$ & 29.5$_9$ & 29.6$_{15}$ & 38.7$_{17}$ & 20.7$_{18}$ & 25.8$_{13}$ \\
    % RoBERTa-base+CRF & 125M & 26.7$_6$ & 39.0$_5$ & 12.5$_4$ & 17.5$_5$ & 18.7$_3$ & 29.3$_1$ & 28.7$_6$ & 39.5$_7$ & 20.1$_{10}$ & 26.8$_{11}$ \\
    \hline
    \multicolumn{8}{l}{(supervised keyphrase generation)} \\
    CatSeq & 21M & 29.1 & 36.7 & 22.5 & 26.2 & 26.9 & 35.4 & 32.3 & 39.7 & 24.2 & 28.3 \\
    ExHiRD-h & 22M & 31.1$_{1}$ & 37.4$_{0}$ & 25.4$_{4}$ & 29.1$_{3}$ & 28.6$_{4}$ & 30.8$_{4}$ & \hfil - \hfil & \hfil - \hfil & 30.4$_{17}$ & 28.2$_{18}$ \\
    Transformer & 98M & 33.3$_{1}$ & 37.6$_{2}$ & 28.8$_{7}$ & 33.3$_{5}$ & 31.4$_{9}$ & 36.5$_{7}$ & 37.8$_{6}$ & 42.9$_{9}$ & 28.8$_{5}$ & 32.1$_{8}$ \\
    SetTrans & 98M & 35.6$_{0}$ & 39.1$_{2}$ & 29.1$_{3}$ & 32.8$_{1}$ & 33.5$_{10}$ & 37.5$_{11}$ & 39.9$_{8}$ & 44.6$_{22}$ & 32.2$_{8}$ & 34.2$_{14}$ \\
    \hdashline
    BERT-G & 110M & 31.3$_{6}$ & 37.9$_{2}$ & 25.9$_{5}$ & 31.3$_{5}$ & 26.3$_{5}$ & 32.2$_{2}$ & 35.2$_{9}$ & 40.9$_{8}$ & 26.3$_{11}$ & 31.0$_{12}$ \\
    % RoBERTa-G & 125M & 28.8$_{5}$ & 36.9$_{3}$ & 22.0$_{5}$ & 27.4$_{7}$ & 23.5$_{6}$ & 31.3$_{12}$ & 30.9$_4$ & 38.1$_{7}$ & 23.3$_{3}$ & 28.6$_{9}$ \\
    SciBERT-G  & 110M & 32.8$_{1}$ & 39.7$_{1}$ & 25.7$_{1}$ & 31.3$_{4}$ & 27.2$_{3}$ & 33.4$_{6}$ & 35.8$_{18}$ & 41.5$_{17}$ & 24.7$_{2}$ & 28.4$_{7}$ \\
    NewsBERT-G & 110M & 29.9$_{5}$ & 36.8$_{2}$ & 26.9$_{7}$ & 32.5$_{8}$ & 25.9$_{6}$ & 31.0$_{9}$ & 33.7$_{9}$ & 39.5$_{10}$ & 24.9$_{13}$ & 29.6$_{15}$ \\    
    UniLM & 110M & 26.7$_{6}$ & 34.6$_{3}$ & 18.2$_{17}$ & 23.6$_{24}$ & 23.5$_{6}$ & 28.5$_{21}$ & 28.4$_{6}$ & 35.3$_{5}$ & 21.5$_{10}$ & 26.8$_{17}$ \\
    B2B-2+10 & 158M & 30.4$_{1}$ & 36.4$_{1}$ & 26.0$_{9}$ & 31.3$_{11}$ & 27.6$_{2}$ & 33.1$_{3}$ & 36.0$_{5}$ & 41.0$_{7}$ & 27.4$_{3}$ & 31.1$_{7}$ \\
    B2B-4+8 & 153M & 31.7$_{1}$ & 37.7$_{2}$ & 26.5$_{5}$ & 31.7$_{6}$ & 27.1$_{10}$ & 32.5$_{5}$ & 35.6$_{3}$ & 40.3$_{6}$ & 26.0$_{16}$ & 30.5$_{17}$ \\
    B2B-6+6 & 148M & 32.1$_{2}$ & 37.7$_{1}$ & 26.7$_{8}$ & 31.7$_{7}$ & 27.3$_{7}$ & 31.6$_{7}$ & 35.4$_{4}$ & 40.3$_{7}$ & 26.4$_{3}$ & 29.8$_{12}$ \\
    B2B-8+4 & 143M & 32.2$_{2}$ & 38.0$_{0}$  & 26.0$_{1}$ & 30.9$_{0}$ & 27.2$_{4}$ & 32.1$_{6}$ & 36.4$_{15}$ & 41.8$_{12}$ & 28.0$_{11}$ & 32.8$_{9}$ \\
    B2B-10+2 & 139M & 31.7$_{2}$ & 38.0$_{2}$  & 26.4$_{8}$ & 31.8$_{11}$ & 26.4$_{6}$ & 31.3$_{8}$ & 34.4$_{22}$ & 39.4$_{16}$ & 26.0$_{20}$ & 30.0$_{15}$\\
    \hdashline
    BART-base & 140M & 32.2$_2$ & 38.8$_3$ & 27.0$_3$ & 32.3$_7$ & 27.0$_6$ & 33.6$_6$ & 36.6$_1$ & 42.4$_8$ & 27.1$_{11}$ & 32.1$_{21}$ \\
    BART-large & 406M & 33.2$_{4}$ & 39.2$_{2}$ & 27.6$_{11}$ & 33.3$_{9}$ & 28.4$_{2}$ & 34.7$_{3}$ & 38.0$_{8}$ & 43.5$_{11}$ & 27.4$_{12}$ & 31.1$_{16}$ \\
    % T5-base & 223M & 33.6$_{1}$ & 38.8$_{0}$ & 28.8$_{5}$ & 33.9$_{5}$ & 30.2$_{3}$ & 35.0$_{2}$ & 38.8$_{6}$ & 44.0$_{4}$ & 29.5$_{16}$ & 32.6$_{16}$ \\
    % T5-large & 770M & 34.3$_{2}$ & 39.3$_{0}$ & 29.5$_{1}$ & 34.3$_{4}$ & 31.5$_{2}$ & 35.9$_{5}$ & 39.8$_{4}$ & 43.8$_{6}$ & 29.7$_{10}$ & 32.1$_{11}$ \\ 
    KeyBART & 406M & 32.5$_{1}$ & 39.8$_{2}$ & 26.8$_{3}$ & 32.5$_{5}$ & 28.7$_{6}$ & 36.5$_{14}$ & 37.3$_{7}$ & 43.0$_{10}$ & 26.0$_{8}$ & 28.9$_{4}$ \\
    SciBART-base & 124M & 34.1$_{1}$ & 39.6$_{2}$ & 27.5$_{10}$ & 32.8$_{8}$ & 28.2$_{8}$ & 32.9$_{11}$ & 37.3$_{7}$ & 42.1$_{14}$ & 27.0$_{8}$ & 30.4$_{8}$ \\
    SciBART-base+OAGKX & 124M & 35.3$_{3}$ & 41.5$_{2}$ & 27.1$_{7}$ & 33.0$_{6}$ & 27.7$_{7}$ & 33.7$_{9}$ & 38.2$_{7}$ & 42.4$_{6}$ & 29.2$_{6}$ & 32.9$_{9}$ \\
    SciBART-large & 386M & 34.7$_{3}$ & 41.5$_{4}$ & 26.1$_{12}$ & 31.7$_{13}$ & 27.1$_{11}$ & 32.4$_{12}$ & 36.4$_{18}$ & 40.9$_{12}$ & 27.9$_{14}$ & 32.0$_{12}$ \\
    SciBART-large+OAGKX & 386M & 36.2$_{1}$ & 43.2$_{0}$ & 26.7$_{5}$ & 33.1$_{4}$ & 28.9$_{8}$ & 34.7$_{6}$ & 38.7$_{11}$ & 44.2$_{11}$ & 30.0$_{7}$ & 33.3$_{19}$ \\
    NewsBART-base & 140M & 32.4$_{3}$ & 38.7$_{2}$ & 26.2$_{10}$ & 31.7$_{11}$ & 26.2$_{8}$ & 32.3$_{15}$ & 36.9$_{8}$ & 42.4$_{10}$ & 26.4$_{21}$ & 30.4$_{23}$ \\
    \hline
    \end{tabular}
    }
    \caption{Present keyphrase evaluation results of all the methods on the SciKP benchmark. The reported results are averaged across three runs with different random seeds. The standard deviation of each entry is presented in the subscript. For example, 23.5$_6$ means an average of 23.5 with a standard deviation of 0.6. We omit the subscript for deterministic methods or methods with a single run.}
    \label{tab:scikp-all-results-pkp}
\end{table*}

\setlength{\tabcolsep}{4pt}
\begin{table*}[!ht]
    % \small
    \centering
    \resizebox{\linewidth}{!} {%
    \begin{tabular}{l | c | l l | l l | l l | l l | l l }
    \hline
    \multirow{2}{*}{Method} &
    \multirow{2}{*}{|M|} & \multicolumn{2}{c|}{\textbf{KP20k}} & \multicolumn{2}{c|}{\textbf{Inspec}} & \multicolumn{2}{c|}{\textbf{Krapivin}} & \multicolumn{2}{c|}{\textbf{NUS}} & \multicolumn{2}{c}{\textbf{SemEval}} \\
    & & F1@5 & F1@M & F1@5 & F1@M & F1@5 & F1@M & F1@5 & F1@M & F1@5 & F1@M\\
    \hline
    CatSeq & 21M & 1.5 & 3.2 & 0.4 & 0.8 & 1.8 & 3.6 & 1.6 & 2.8 & 2.0 & 2.8 \\
    ExHiRD-h & 22M & 1.6$_{0}$ & 2.5$_{0}$ & 1.1$_{1}$ & 1.6$_{2}$ & 2.2$_{3}$ & 3.3$_{4}$ & \hfil - \hfil & \hfil - \hfil & 1.6$_{4}$ & 2.1$_{6}$ \\
    Transformer & 98M & 2.2$_{2}$ & 4.6$_{4}$ & 1.2$_{0}$ & 2.3$_{1}$ & 3.3$_{2}$ & 6.3$_{4}$ & 2.5$_{4}$ & 4.4$_{9}$ & 1.6$_{2}$ & 2.2$_{4}$ \\
    SetTrans & 98M & 3.5$_{1}$ & 5.8$_{1}$ & 1.9$_{1}$ & 3.0$_{1}$ & 4.5$_{1}$ & 7.2$_{3}$ & 3.7$_{10}$ & 5.5$_{17}$ & 2.2$_{2}$ & 2.9$_{2}$ \\
    \hdashline
    BERT-G & 110M  & 1.9$_{1}$ & 3.7$_{2}$ & 1.0$_{2}$ & 1.9$_{6}$ & 2.4$_{2}$ & 4.3$_{4}$ & 2.2$_{5}$ & 3.9$_{11}$ & 1.4$_{2}$ & 2.0$_{3}$ \\
    % RoBERTa-G & 125M & 2.0$_{0}$ & 3.1$_{0}$ & 1.0$_{1}$ & 2.0$_2$ & 2.7$_2$ & 4.8$_3$ & 2.5$_4$ & 4.3$_8$ & 2.1$_1$ & 2.9$_1$ \\
    SciBERT-G & 110M & 2.4$_{0}$ & 4.6$_{1}$ & 1.4$_{2}$ & 2.7$_{5}$ & 2.4$_{3}$ & 4.6$_{5}$ & 3.4$_{9}$ & 5.9$_{18}$& 1.3$_{1}$ & 1.8$_{2}$ \\
    NewsBERT-G & 110M & 1.3$_{1}$ & 2.6$_{3}$ & 0.8$_{2}$ & 1.5$_{4}$ & 1.7$_{2}$ & 3.4$_{2}$ & 1.5$_{2}$ & 2.8$_{6}$ & 1.3$_{2}$ & 1.9$_{3}$ \\
    UniLM & 110M & 1.4$_{2}$ & 2.8$_{4}$ & 0.5$_{1}$ & 0.8$_{2}$ & 1.4$_{3}$ & 2.4$_{5}$ & 1.7$_{3}$ & 3.2$_{7}$ & 1.0$_{4}$ & 1.5$_{6}$ \\
    B2B-2+10 & 158M & 2.1$_{1}$ & 3.9$_{1}$ & 1.1$_{2}$ & 1.9$_{3}$ & 2.7$_{4}$ & 4.7$_{6}$ & 2.8$_{5}$ & 4.7$_{7}$ & 1.9$_{1}$ & 2.6$_{2}$ \\
    B2B-4+8 & 153M & 2.2$_{1}$ & 4.1$_{1}$ & 1.1$_{1}$ & 2.0$_{1}$ & 2.6$_{1}$ & 4.4$_{1}$ & 2.7$_{5}$ & 4.3$_{6}$ & 2.2$_{2}$ & 2.9$_{3}$ \\
    B2B-6+6 & 148M & 2.2$_{2}$ & 4.1$_{2}$ & 1.0$_{3}$ & 1.8$_{5}$ & 2.7$_{1}$ & 4.6$_{1}$ & 2.8$_{5}$ & 4.2$_{5}$ & 1.7$_{8}$ & 2.3$_{9}$ \\
    B2B-8+4 & 143M & 2.2$_{1}$ & 4.2$_{1}$ & 1.1$_{0}$ & 2.0$_{1}$ & 2.8$_{3}$ & 5.2$_{5}$ & 2.6$_{8}$ & 4.1$_{15}$ & 1.8$_{3}$ & 2.3$_{3}$ \\
    B2B-10+2 & 139M & 2.1$_{1}$ & 4.1$_{2}$ & 1.2$_{4}$ & 2.3$_{8}$ & 2.4$_{3}$ & 4.4$_{4}$ & 2.6$_{6}$ & 4.6$_{13}$ & 1.8$_{4}$ & 2.5$_{5}$ \\
    \hdashline
    BART-base & 140M & 2.2$_1$ & 4.2$_2$ & 1.0$_1$ & 1.7$_2$ & 2.8$_3$ & 4.9$_6$ & 2.6$_4$ & 4.2$_9$ & 1.6$_1$ & 2.1$_2$ \\
    BART-large & 406M & 2.7$_{2}$ & 4.7$_{2}$ & 1.5$_{3}$ & 2.4$_{4}$ & 3.1$_{1}$ & 5.1$_{2}$ & 3.1$_{5}$ & 4.8$_{9}$ & 1.9$_{3}$ & 2.4$_{3}$ \\
    % T5-base & 223M & 1.7$_{0}$ & 3.4$_{0}$ & 1.1$_{1}$ & 2.0$_{3}$ & 2.3$_{2}$ & 4.3$_{4}$ & 2.7$_{0}$ & 5.1$_{3}$ & 1.4$_{4}$ & 2.0$_{5}$ \\
    % T5-large & 770M & 1.7$_{0}$ & 3.5$_{0}$ & 1.1$_{3}$ & 2.1$_{6}$ & 2.3$_{4}$ & 4.5$_{7}$ & 2.5$_{3}$ & 4.2$_{6}$ & 1.5$_{1}$ & 2.0$_{3}$ \\ 
    KeyBART & 406M & 2.6$_{1}$ & 4.7$_{1}$ & 1.4$_{2}$ & 2.3$_{2}$ & 3.6$_{2}$ & 6.4$_{6}$ & 3.1$_{4}$ & 5.5$_{7}$ & 1.6$_{4}$ & 2.2$_{5}$ \\
    SciBART-base & 124M & 2.9$_{3}$ & 5.2$_{4}$ & 1.6$_{2}$ & 2.8$_{4}$ & 3.3$_{4}$ & 5.4$_{8}$ & 3.3$_{1}$ & 5.3$_{2}$ & 1.8$_{1}$ & 2.2$_{1}$ \\
    SciBART-base+OAGKX & 124M & 2.8$_{1}$ & 5.2$_{1}$ & 1.5$_{3}$ & 2.7$_{4}$ & 3.2$_{4}$ & 5.7$_{7}$ & 2.8$_{1}$ & 4.8$_{2}$ & 1.8$_{0}$ & 2.4$_{0}$ \\
    SciBART-large & 386M & 3.1$_{2}$ & 5.7$_{3}$ & 1.5$_{2}$ & 2.6$_{2}$ & 3.4$_{1}$ & 5.6$_{3}$ & 3.2$_{5}$ & 5.0$_{7}$ & 2.6$_{6}$ & 3.3$_{8}$ \\
    SciBART-large+OAGKX & 386M & 3.2$_{1}$ & 6.2$_{1}$ & 1.7$_{1}$ & 3.0$_{1}$ & 3.6$_{2}$ & 6.4$_{7}$ & 3.3$_{2}$ & 5.5$_{5}$ & 2.3$_{1}$ & 3.1$_{2}$ \\
    NewsBART-base & 140M & 2.2$_{1}$ & 4.4$_{2}$ & 1.0$_{1}$ & 1.8$_{2}$ & 2.4$_{2}$ & 4.5$_{4}$ & 2.4$_{4}$ & 4.0$_{9}$ & 1.6$_{1}$ & 2.2$_{2}$ \\
    \hline
    \end{tabular}
    }
    % \vspace{-2mm}
    \caption{Absent keyphrase evaluation results of all keyphrase generation methods on the SciKP benchmark. The standard deviation of each entry is presented in the subscript. For example, 23.5$_6$ means an average of 23.5 with a standard deviation of 0.6. We omit the subscript for deterministic methods or methods with a single run.}
    \label{tab:scikp-all-results-akp}
    % \vspace{-2mm}
\end{table*}

\setlength{\tabcolsep}{4pt}
\begin{table*}[]
    % \small
    \centering
    \begin{tabular}{l | c | l l | l l }
    \hline
    \multirow{2}{*}{Method} &
    \multirow{2}{*}{|M|} & \multicolumn{2}{c|}{\textbf{KPTimes}} & \multicolumn{2}{c}{\textbf{StackEx}} \\
     & & F1@5 & F1@M & F1@5 & F1@M \\
    \hline
    \multicolumn{4}{l}{(keyphrase extraction baselines)} \\
    KP-Miner & - & 18.0 & \hfil - \hfil & 16.8 & \hfil - \hfil \\
    YAKE & - & 13.1 & \hfil - \hfil & 13.0 & \hfil - \hfil \\
    TextRank & - & 17.4 & \hfil - \hfil & 12.6 & \hfil - \hfil \\
    PositionRank & - & 11.9 & \hfil - \hfil & 12.1 & \hfil - \hfil \\
    MultipartiteRank & - & 19.5 & \hfil - \hfil & 13.7 & \hfil - \hfil \\
    EmbedRank & - & 10.2 & \hfil - \hfil & 11.4 & \hfil - \hfil \\
    SIFRank+ & - & 15.8 & \hfil - \hfil & 12.0  & \hfil - \hfil \\
    \citet{liang-etal-2021-unsupervised} & - & 16.2 & \hfil - \hfil & 13.8 & \hfil - \hfil \\
    Kea & - & 18.3 & \hfil - \hfil & 17.8 & \hfil - \hfil \\
     \hline
     \multicolumn{4}{l}{(supervised keyphrase extraction)} \\
    Transformer & 110M & 28.8$_{5}$ & 42.7$_{5}$ & 25.1$_{9}$ & 48.7$_{11}$ \\
    Transformer+CRF & 110M & 28.2$_{6}$ & 43.2$_{3}$ & 26.0$_{8}$ & 52.0$_{11}$ \\
    BERT-base & 110M &  34.0$_{4}$ & 49.3$_{3}$ & 29.0$_{8}$ & 56.8$_{9}$ \\
    BERT-base+CRF & 110M &  33.9$_{7}$ & 49.9$_{6}$ & 28.5$_{5}$ & 56.3$_{5}$ \\
    SciBERT & 110M  & 31.8$_{3}$ & 47.7$_{2}$ & 29.2$_{5}$ & 57.5$_{5}$ \\
    SciBERT+CRF & 110M &  31.8$_{6}$ & 48.1$_{5}$ & 28.6$_{3}$ & 57.1$_{3}$ \\
    NewsBERT & 110M & 34.5$_{5}$ & 50.4$_{4}$ & 28.5$_{3}$ & 56.2$_{2}$ \\
    NewsBERT+CRF & 110M & 34.9$_{4}$ & 50.8$_{5}$ & 28.5$_{2}$ & 56.2$_{2}$ \\
    % RoBERTa-base & 125M & 33.2$_{2}$ & 48.9$_{2}$ & 28.7$_{2}$ & 56.2$_{5}$ \\
    % RoBERTa-base+CRF & 125M & 32.4$_{6}$ & 48.4$_{3}$ & 27.6$_{10}$ & 55.4$_{10}$ \\
    \hline
    \multicolumn{4}{l}{(supervised keyphrase generation)} \\
    CatSeq & 21M & 29.5 & 45.3 & \hfil - \hfil & \hfil - \hfil \\
    ExHiRD-h & 22M & 32.1$_{16}$ & 45.2$_{7}$ & 28.8$_{2}$ & 54.8$_{2}$ \\
    Transformer & 98M & 30.2$_{5}$ & 45.3$_{6}$ & 30.8$_{5}$ & 55.4$_{2}$ \\
    SetTrans & 98M & 35.6$_{5}$ & 46.3$_{4}$ & 35.8$_{3}$ & 56.7$_{5}$ \\
    \hdashline
    BERT-G & 110M & 32.3$_{5}$ & 47.4$_{3}$ & 28.5$_{6}$ & 54.9$_{6}$ \\
    SciBERT-G & 110M & 33.0$_{1}$ & 48.4$_{1}$ & 29.5$_{3}$ & 56.5$_{1}$ \\
    NewsBERT-G & 110M & 33.0$_{2}$ & 48.0$_{1}$ & 28.8$_{1}$ & 55.3$_{0}$ \\
    % RoBERTa-G & 125M & 33.0$_{2}$ & 48.2$_{5}$ & \hfil - \hfil & \hfil - \hfil \\
    UniLM & 110M & 33.2$_{3}$ & 48.0$_{2}$ & \hfil - \hfil & \hfil - \hfil \\
    B2B-2+10 & 158M & 31.6$_{5}$ & 46.5$_{6}$ & 28.8$_{}$ & 55.4$_{}$ \\
    B2B-4+8 & 153M & 32.9$_{2}$ & 47.6$_{1}$ & 29.4$_{}$ & 55.7$_{}$ \\
    B2B-6+6 & 148M & 33.8$_{2}$ & 48.4$_{2}$ & 29.0$_{}$ & 55.6$_{}$ \\
    B2B-8+4 & 143M & 33.8$_{4}$ & 48.6$_{2}$ & 28.6$_{}$ & 55.6$_{}$ \\
    B2B-10+2 & 139M & 33.5$_{4}$ & 48.4$_{4}$ & 29.1$_{}$ & 55.9$_{}$ \\
    \hdashline
    BART-base & 140M & 35.9$_{1}$ & 49.9$_{2}$ & 30.4$_{1}$ & 57.1$_{1}$ \\
    BART-large & 406M & 37.3$_{16}$ & 51.0$_{15}$ & 31.2$_{2}$ & 57.8$_{8}$ \\
    % T5-base & 223M & 34.6$_{2}$ & 49.2$_{2}$ & 28.7$_{1}$ & 56.1$_{1}$ \\
    % T5-large & 770M & 36.6$_{0}$ & 50.8$_{1}$ & 30.5$_{2}$ & 58.0$_{3}$ \\
    KeyBART & 406M & 37.8$_{6}$ & 51.3$_{1}$ & 31.9$_{5}$ & 58.9$_{2}$ \\
    SciBART-base & 124M & 34.8$_{4}$ & 48.8$_{1}$ & 30.4$_{6}$ & 57.6$_{4}$ \\
    SciBART-large & 386M & 35.3$_{4}$ & 49.7$_{2}$ & 30.9$_{3}$ & 57.8$_{2}$ \\
    SciBART-large+OAGKX & 386M & 35.6$_{8}$ & 50.0$_{3}$ & 31.8$_{0}$ & 58.5$_{3}$ \\
    NewsBART-base & 140M & 35.4$_{2}$ & 49.8$_{1}$ & 30.7$_{3}$ & 57.5$_{0}$ \\
    \hline
    \end{tabular}
    % \vspace{-2mm}
    \caption{Present keyphrase evaluation results of all the methods on KPTimes and StackEx. The reported results are averaged across three runs with different random seeds. The standard deviation of each entry is presented in the subscript. For example, 23.5$_6$ means an average of 23.5 with a standard deviation of 0.6. We omit the subscript for deterministic methods or methods with a single run.}
    \label{tab:other-all-results-pkp}
    % \vspace{-2mm}
\end{table*}

\setlength{\tabcolsep}{4pt}
\begin{table*}[]
    % \small
    \centering
    % \resizebox{\linewidth}{!}{%
    \begin{tabular}{l | c | l l | l l }
    \hline
    \multirow{2}{*}{Method} &
    \multirow{2}{*}{|M|} & \multicolumn{2}{c|}{\textbf{KPTimes}} & \multicolumn{2}{c}{\textbf{StackEx}} \\
     &  & F1@5 & F1@M & F1@5 & F1@M \\
    \hline
    CatSeq & 21M & 15.7 & 22.7 & \hfil - \hfil & \hfil - \hfil \\
    ExHiRD-h & 22M & 13.4$_{2}$ & 16.5$_{1}$ & 10.1$_{1}$ & 15.5$_{1}$ \\
    Transformer & 98M & 17.1$_{1}$ & 23.1$_{1}$ & 10.4$_{2}$ & 18.7$_{2}$ \\
    SetTrans & 98M & 19.8$_{3}$ & 21.9$_{2}$ & 13.9$_{1}$ & 20.7$_{0}$ \\
    \hdashline
    BERT-G & 110M & 16.5$_{7}$ & 24.6$_{5}$ & 10.7$_{8}$ & 22.8$_{10}$ \\
    SciBERT-G & 110M & 15.7$_{2}$ & 24.7$_{0}$ & 11.8$_{5}$ & 24.8$_{7}$ \\
    NewsBERT-G & 110M & 17.0$_{5}$ & 25.6$_{1}$ & 11.7$_{1}$ & 24.5$_{1}$ \\
    % RoBERTa-G & 125M & 17.1$_{2}$ & 25.5$_{3}$ & \hfil - \hfil & \hfil - \hfil \\
    UniLM & 110M & 15.2$_{10}$ & 24.1$_{11}$ & \hfil - \hfil & \hfil - \hfil \\
    B2B-2+10 & 158M & 16.2$_{4}$ & 23.2$_{0}$ & 10.7$_{}$ & 22.3$_{}$ \\
    B2B-4+8 & 153M & 15.9$_{1}$ & 23.6$_{3}$ & 11.2$_{}$ & 22.8$_{}$ \\
    B2B-6+6 & 148M & 16.4$_{3}$ & 24.1$_{1}$ & 11.1$_{}$ & 22.9$_{}$ \\
    B2B-8+4 & 143M & 16.8$_{2}$ & 24.5$_{1}$ & 10.5$_{}$ & 22.2$_{}$ \\
    B2B-10+2 & 139M & 16.8$_{1}$ & 24.5$_{2}$ & 11.1$_{}$ & 23.4$_{}$ \\
    \hdashline
    BART-base & 140M & 17.1$_{2}$ & 24.9$_{1}$ & 11.7$_{0}$ & 24.9$_{2}$ \\
    BART-large & 406M & 17.6$_{10}$ & 24.4$_{19}$ & 12.4$_{1}$ & 26.1$_{3}$ \\
    % T5-base & 223M & 15.3$_{1}$ & 24.2$_{1}$ & 9.4$_{0}$ & 21.6$_{1}$ \\
    % T5-large & 770M & 15.7$_{1}$ & 24.1$_{1}$ & 10.6$_{1}$ & 23.9$_{2}$ \\
    KeyBART & 406M & 18.0$_{7}$ & 25.5$_{2}$ & 13.0$_{5}$ & 27.1$_{5}$ \\
    SciBART-base & 124M & 17.2$_{3}$ & 24.6$_{2}$ & 11.1$_{6}$ & 24.2$_{8}$ \\
    SciBART-large & 386M & 17.2$_{3}$ & 25.7$_{2}$ & 12.6$_{1}$ & 26.7$_{1}$ \\
    SciBART-large+OAGKX & 386M & 17.4$_{4}$ & 25.8$_{4}$ & 13.4$_{3}$ & 27.9$_{3}$ \\
    NewsBART-base & 140M & 17.6$_{3}$ & 26.1$_{1}$ & 12.1$_{3}$ & 25.7$_{4}$ \\
    \hline
    \end{tabular}
    % }
    % \vspace{-2mm}
    \caption{Absent keyphrase evaluation results of all the methods on KPTimes and StackEx. The standard deviation of each entry is presented in the subscript. For example, 23.5$_6$ means an average of 23.5 with a standard deviation of 0.6. We omit the subscript for deterministic methods or methods with a single run.}
    \label{tab:other-all-results-akp}
    % \vspace{-2mm}
\end{table*}
