# Supplementary material for: On Leveraging Encoder-only Pre-trained Language Models for Effective Keyphrase Generation
Source: arXiv:2402.14052 source file (2024-02-21)
Supplement: Supplementary file 2 [file qual_ex1.tex]

\begin{figure*}[h!]
\small
\centering
\begin{tabular}{p{0.98\linewidth}}
    \hline  
    \textbf{Title:} a review of \textcolor{blue}{design pattern} mining techniques . \\
    \textbf{Abstract:} the quality of a software system highly depends on its architectural design . high quality software systems typically apply expert design experience which has been captured as \textcolor{blue}{design patterns} . as demonstrated solutions to recurring problems , \textcolor{blue}{design patterns} help to reuse expert experience in software system design . they have been extensively applied in the industry . mining the instances of \textcolor{blue}{design patterns} from the source code of software systems can assist in the understanding of the systems and the process of re engineering them . more importantly , it also helps to trace back to the original design decisions , which are typically missing in legacy systems . this paper presents a review on current techniques and tools for mining \textcolor{blue}{design patterns} from source code or design of software systems . we classify different approaches and analyze their results in a comparative study . we also examine the disparity of the \textcolor{blue}{discovery} results of different approaches and analyze possible reasons with some insight . \\
    \hdashline
    \textbf{Ground Truth:} \textcolor{blue}{design pattern}, \textcolor{blue}{discovery}, \textcolor{blue}{reverse engineering}
\\
    \hdashline
    \textbf{BART:} unrelated scheduling, mechanism design, approximation algorithms  \\
    % \textbf{T5:} \textcolor{blue}{design patterns}, software architecture, software design, software reuse  \\
    \textbf{SciBERT:} \textcolor{blue}{design patterns}, software systems, software engineering, software mining \\
    \textbf{SciBART:} design pattern mining, software system design, \textcolor{blue}{reverse engineering}, software reuse \\
    \textbf{KeyBART:} \textcolor{blue}{design patterns}, software architecture, software reuse, software quality, software maintenance \\
    \hline
    \hline  
    \textbf{Title:} stabilization of \textcolor{blue}{second order nonholonomic systems} in canonical chained form .  \\
    \textbf{Abstract:} stabilization of a class of \textcolor{blue}{second order nonholonomic systems} in canonical chained form is investigated in this paper . first , the models of two typical \textcolor{blue}{second order nonholonomic systems} , namely , a three link planar manipulator with the third joint unactuated , and a kinematic redundant manipulator with all joints free and driven by forces torques imposing on the end effector , are presented and converted to second order chained form by transformations of coordinate and input . a discontinuous control law is then proposed to stabilize all states of the system to the desired equilibrium point exponentially . computer simulation is given to show the effectiveness of the proposed controller . \\
    \hdashline
    \textbf{Ground Truth:} \textcolor{blue}{second order nonholonomic systems}, \textcolor{blue}{canonical second order chained form}, \textcolor{blue}{underactuated manipulator}, \textcolor{blue}{discontinuous coordinate transformation}, \textcolor{blue}{discontinuous stabilization}
\\
    \hdashline
    \textbf{BART:} stabilization, \textcolor{blue}{second order nonholonomic systems}, canonical chained form, discontinuous control law   \\
    % \textbf{T5:} stabilization, \textcolor{blue}{second order nonholonomic system}, canonical chained form, discontinuous control \\
    \textbf{SciBERT:} stabilization, nonholonomic system, canonical chained form, redundant manipulator \\
    \textbf{SciBART:} stabilization, \textcolor{blue}{second order nonholonomic systems}, canonical chained form, discontinuous control law \\
    \textbf{KeyBART:} stabilization, \textcolor{blue}{second order nonholonomic systems}, discontinuous control law \\
    \hline
    \hline
    \textbf{Title:} characterizing output processes of e m e k [digit] queues . \\
    \textbf{Abstract:} our goal is to study which conditions of the output process of a queue preserve the increasing failure rate ( \textcolor{blue}{ifr} ) property in the interdeparture time . we found that the interdeparture time does not always preserve the \textcolor{blue}{ifr} property , even if the interarrival time and service time are both \textcolor{blue}{erlang distributions} with \textcolor{blue}{ifr} . we give a theoretical analysis and present numerical results of e m e k [digit] queues . we show , by numerical examples , that the interdeparture time of e m e k [digit] retains the \textcolor{blue}{ifr} property if m > k. ( c ) [digit] elsevier ltd. all rights reserved .\\
    \hdashline
    \textbf{Ground Truth:} \textcolor{blue}{ifr}, \textcolor{blue}{erlang distribution}, \textcolor{blue}{departure process}, \textcolor{blue}{ph g [digit]}, \textcolor{blue}{queueing theory} \\
    \hdashline
    \textbf{BART:} output process, increasing failure rate, interdeparture time, \textcolor{blue}{erlang distribution} \\
    % \textbf{T5:} output process, increasing failure rate, \textcolor{blue}{erlang distribution} \\
    \textbf{SciBERT:} increasing failure rate, interdeparture time, \textcolor{blue}{erlang distribution}, output process of a queue \\
    \textbf{SciBART:} output process, increasing failure rate, interdeparture time, \textcolor{blue}{erlang distribution}, \textcolor{blue}{queueing theory} \\
    \textbf{KeyBART:} output process, increasing failure rate, interdeparture time, \textcolor{blue}{erlang distribution}, \textcolor{blue}{queueing theory} \\
    \hline
    \hline  
    \textbf{Title:} optimal tool selection for \textcolor{blue}{2.5 d milling} , part [digit] a \textcolor{blue}{solid modeling approach} for construction of the voronoi mountain \\
    \textbf{Abstract:} \textcolor{blue}{cutter selection} is a critical subtask of machining process planning . in this two part series , we develop a robust approach for the selection of an optimal set of milling cutters for a 2.5 d generalized pocket . in the first article ( part [digit] ) , we present a \textcolor{blue}{solid modeling} approach for the construction of the \textcolor{blue}{voronoi mountain} for the pocket geometry , which is a 3d extension of the voronoi diagram . the major contributions of this work include ( [digit] ) the development of a robust and systematic procedure for construction of the \textcolor{blue}{voronoi mountain} for a multiply connected curvilinear polygon and ( b ) an extension of the \textcolor{blue}{voronoi mountain} concept to handle \textcolor{blue}{open edges} . \\
    \hdashline
    \textbf{Ground Truth:} \textcolor{blue}{2.5 d milling}, \textcolor{blue}{solid modelling}, \textcolor{blue}{voronoi mountain}, \textcolor{blue}{cutter selection}, \textcolor{blue}{open edges} \\
    \hdashline
    \textbf{BART:} \textcolor{blue}{solid modeling}, \textcolor{blue}{voronoi mountain}, \textcolor{blue}{cutter selection}, 2.5 d generalized pocket, curve generation  \\
    % \textbf{T5:} tool selection, \textcolor{blue}{2.5 d milling}, voronoi diagram, machining geometry\\
    \textbf{SciBERT:} tool selection, milling, \textcolor{blue}{voronoi mountain}, pocket geometry, cutter path planning \\
    \textbf{SciBART:} tool selection, \textcolor{blue}{2.5 d milling}, \textcolor{blue}{voronoi mountain}, \textcolor{blue}{cutter selection}, voronoi diagram, pocket milling \\
    \textbf{KeyBART:} tool selection, \textcolor{blue}{2.5 d milling}, \textcolor{blue}{voronoi mountain}, process planning, generalized pocket, vlsi cad cam \\
    \hline
\end{tabular}
\caption{Example outputs from various PLMs on the SciKP benchmarks. Correct keyphrases are colored in \textcolor{blue}{blue}.}
\label{example-outputs-kp20k}
\end{figure*}
