# Supplementary material for: On Leveraging Encoder-only Pre-trained Language Models for Effective Keyphrase Generation
Source: arXiv:2402.14052 source file (2024-02-21)
Supplement: Supplementary file 3 [file num_kp_results.tex]

\setlength{\tabcolsep}{3.5pt}
\begin{table*}[]
    \small
    \centering
    \begin{tabular}{l | c | c | c | c | c | c | c | c }
    \hline
    Method & \textbf{KP20k} & \textbf{Inspec} & \textbf{Krapivin} & \textbf{NUS} & \textbf{SemEval} & \textbf{KPTimes} & \textbf{OpenKP} & \textbf{StackEx} \\
    \hline
    Reference &  &  &  &  &  &  & & \\
    \hline
    \multicolumn{6}{l}{(supervised, sequence tagging)} \\
    BERT-base  &  &  &  &  &  &  &  &   \\
    BERT-base+CRF  &  &  &  &  &  &  &  &   \\
    RoBERTa  &  &  &  &  &  &  &  &   \\
    RoBERTa+CRF  &  &  &  &  &  &  &  &   \\
    SciBERT  &  &  &  &  &  &  &  &   \\
    SciBERT+CRF  &  &  &  &  &  &  &  &   \\
    \hline
    \multicolumn{6}{l}{(supervised, sequence generation via mask manipulation)} \\
    BERT-base \\
    SciBERT \\
    RoBERTa-base \\
    UniLM \\
    \hline
    \multicolumn{4}{l}{(supervised, sequence generation)} \\
     &  &  &  &  &  &  &  &   \\
     &  &  &  &  &  &  &  & \\
    BART-base & &  &  &  &  &  &  & \\
    \hline
    \multicolumn{4}{l}{(supervised, no pre-training)} \\
    Kea  &  &  &  &  &  &  &  & \\
    ExHiRD-h  &  &  &  &  &  &  &  & \\
    One2Set  &  &  &  &  &  &  &  & \\
    \hline
    \end{tabular}
    % \vspace{-2mm}
    \caption{Average number of generated keyphrases and their mean squared error compared to the ground truth label.}
    \label{tab:num-kp-results}
    % \vspace{-2mm}
\end{table*}
