# Supplementary material for: On Leveraging Encoder-only Pre-trained Language Models for Effective Keyphrase Generation
Source: arXiv:2402.14052 source file (2024-02-21)
Supplement: Supplementary file 4 [file scibart-summ-results.tex]

\begin{table*}[h!]
\small 
\centering
% \resizebox{\columnwidth}{!}{
\begin{tabular}{l | c c c c c}
\hline
 & \multicolumn{2}{c}{arXiv} && \multicolumn{2}{c}{PubMed} \\
\cline{2-3}\cline{5-6}
\textbf{Model} & Rouge-1/2/L & BERTScore && Rouge-1/2/L & BERTscore \\
\hline
BART-base & 37.03/11.46/33.18 & 0.3294 && 39.85/15.63/37.17 & 0.3888\\
SciBART-base & 38.19/12.21/34.30 & 0.3416 && 40.54/16.19/37.76 & 0.3956 \\
\hdashline
BART-large & 38.58/12.23/34.68 & 0.3416 && 41.18/16.55/38.47 & 0.4003 \\
SciBART-large & \textbf{39.03}$^\dagger$/\textbf{12.60}$^\dagger$/\textbf{35.17}$^\dagger$ & \textcolor{white}{1}\textbf{0.3459}$^\dagger$ && \textbf{41.71}$^\dagger$/\textbf{16.99}$^\dagger$/\textbf{38.93}$^\dagger$ & \textcolor{white}{1}\textbf{0.4080}$^\dagger$ \\
\\
 & \multicolumn{2}{c}{MEDIQA-QS} && \multicolumn{2}{c}{MEDIQA-MAS}\\
\cline{2-3}\cline{5-6}
 & Rouge-1/2/L & BERTScore && Rouge-1/2/L & BERTScore \\
\hline
BART-base & 28.82/10.99/26.99 & 0.8960 && 31.63/9.98/27.85 & 0.8590 \\
BioBART-base & 29.97/10.64/28.41 & 0.9010 && 29.32/9.00/26.14 & 0.8570 \\
SciBART-base & 29.17/11.19/27.53 & 0.8995 && 33.35/11.41/29.92 & 0.8627 \\
\hdashline
BART-large & 30.12/11.28/27.44 & 0.8980 && 32.90/11.28/29.26 & 0.8610 \\
BioBART-large & 31.97/\textbf{12.39}/\textbf{29.70} & 0.9030 && 30.60/11.37/27.04 & 0.8610 \\
SciBART-large & \textbf{32.88}$^\dagger$/12.34/29.66 & \textbf{0.9037} && \textcolor{white}{1}\textbf{35.21}$^\dagger$/\textbf{13.12}$^\dagger$/\textbf{31.86}$^\dagger$ & \textcolor{white}{1}\textbf{0.8680}$^\dagger$ \\
\hline
\end{tabular}
% }
\caption{Experiment results on summarization. SciBART-large achieves the best performance on the majority of the datasets. $^\dagger$ indicates statistically significantly higher than the second best model.}
\label{tab:results-summarization}
\vspace{-2mm}
\end{table*}
