# Supplementary material for: On Leveraging Encoder-only Pre-trained Language Models for Effective Keyphrase Generation
Source: arXiv:2402.14052 source file (2024-02-21)
Supplement: Supplementary file 5 [file t5_prefixes.tex]

\setlength{\tabcolsep}{3.5pt}
\begin{table}[h]
    % \small
    \centering
    \resizebox{\linewidth}{!}{%
    \begin{tabular}{l | c c | c c  }
    \hline
    \multirow{2}{*}{Prefix} & \multicolumn{2}{c|}{\textbf{Present KPs}} & \multicolumn{2}{c}{\textbf{Absent KPs}} \\
    & F1@5 & F1@M & F1@5 & F1@M \\
    \hline
    \texttt{summarize:} & 33.6 & 38.8 & \textbf{1.7} & \textbf{3.4} \\
    \hdashline
    \begin{tabular}[x]{@{}l}\texttt{generate}\\\texttt{keyphrases:}\end{tabular} & \textbf{33.7} & \textbf{38.9} & \textbf{1.7} & \textbf{3.4} \\
    \hdashline
    \texttt{None} & 33.5 & 37.9 & 1.4 & 2.9 \\
    \hline
    \end{tabular}
    }
    % \vspace{-2mm}
    \caption{
    Comparison across different prefixes for fine-tuning T5. We use T5-base for all experiments and report the averaged scores across three runs. 
    }
    \label{tab:t5-prefixes}
    % \vspace{-2mm}
\end{table}
